# Supplementary material for: Speech2Face: Learning the Face Behind a Voice
Source: arXiv:1905.09773 source file (2019-05-23)
Supplement: Supplementary file 1 [file sec6_supplementary.tex]

\cleardoublepage
% \setcounter{page}{1}
% \maketitle
% \usepackage{caption}
% \twocolumn[{%
% \renewcommand\twocolumn[1][]{#1}%
\maketitle
% \begin{center}
%     \centering
%     \includegraphics[width=.8\textwidth,height=5cm]{example-image}
%     \captionof{figure}{Test caption}
% \end{center}%
% }]

\section*{Contents}
This supplementary material contains additional information that could not be included in the main paper due to the space limitation:
\begin{itemize} 
 \item Attribute evaluation for reference between original image v.s. face reconstruction from face feature.
 \item t-SNE visualization of AVSpeech test samples.
\end{itemize}

A separate HTML supplementary material contains the following information:
\begin{itemize} 
 \item The additional qualitative results of AVSpeech test samples. 
 \item The qualitative results of image retrieval.
\end{itemize}

\subsection*{Attribute evaluation for reference}
\figref{attr_eval_f2f}

\begin{figure*}[t]
\def\attrszgender{0.45\linewidth}
\def\attrszage{0.8\linewidth}
\def\attrszethnicity{0.54\linewidth}
\centering
\vspace{-3mm}
\resizebox{1\linewidth}{!}{
% \scriptsize
\includegraphics[width=\attrszgender]{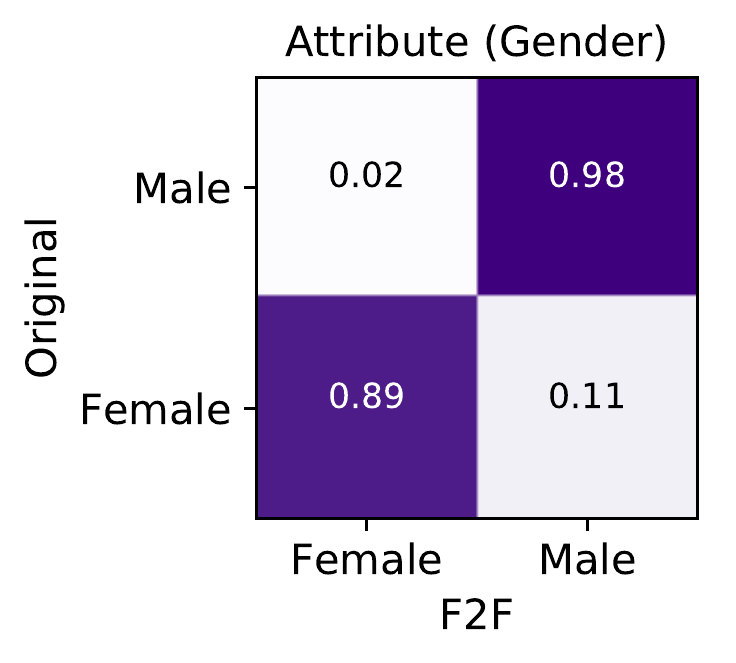}
\includegraphics[width=\attrszethnicity]{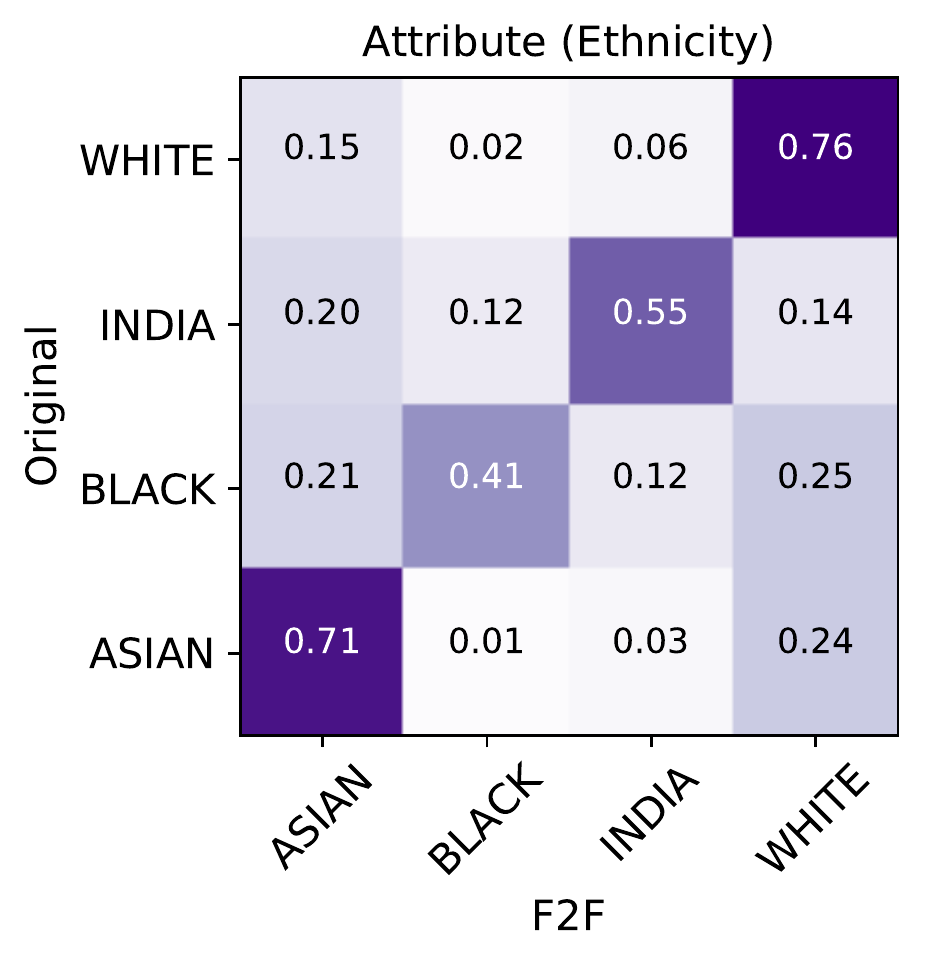}
\includegraphics[width=\attrszage]{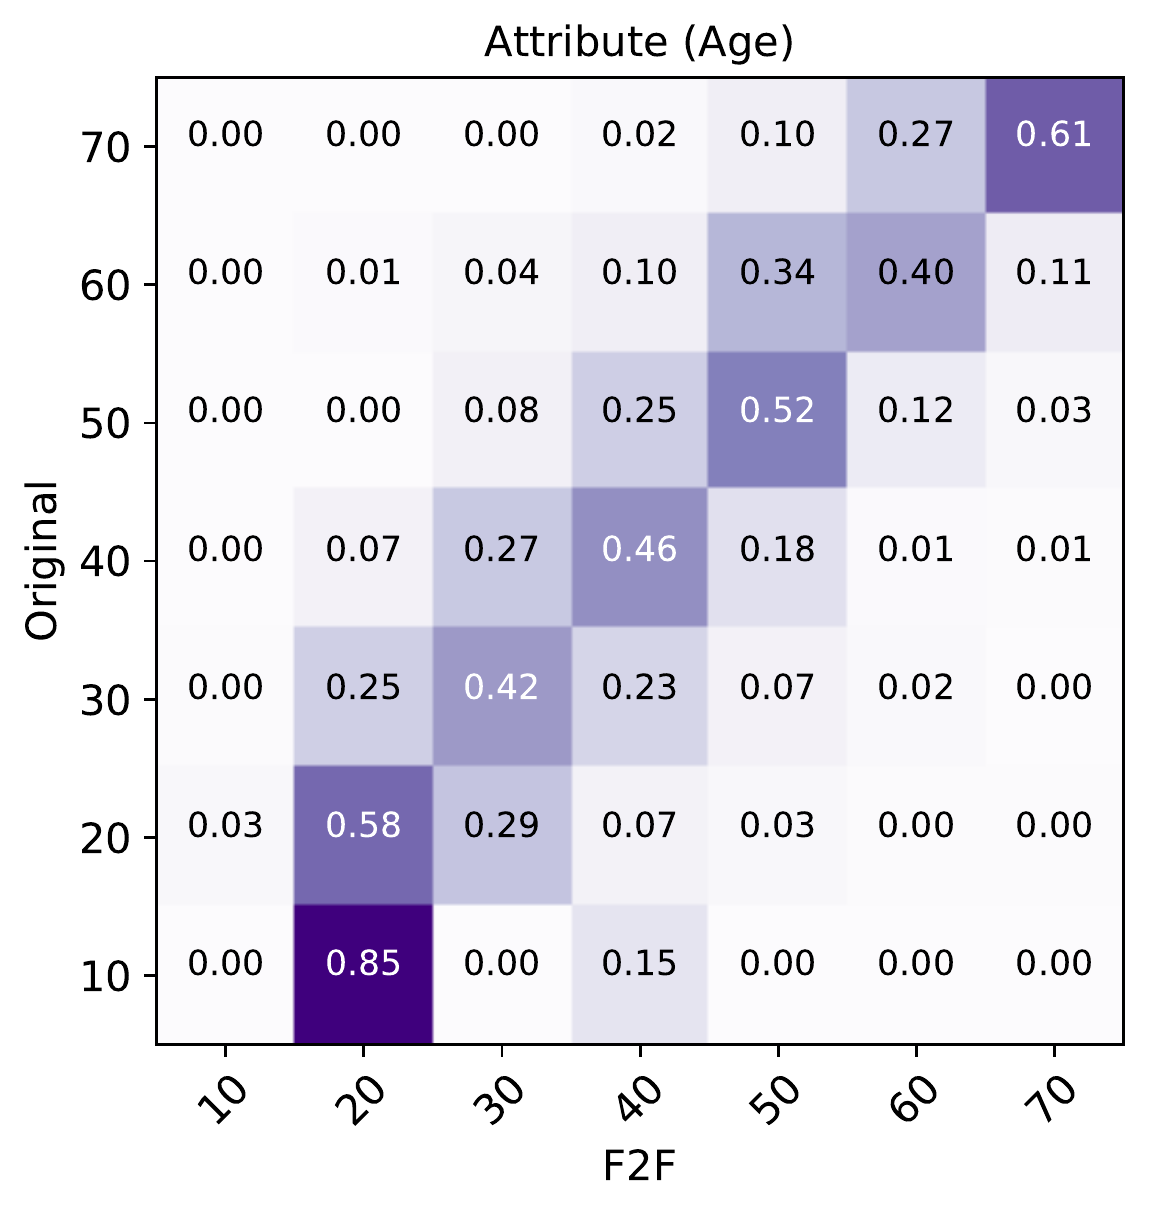}
        % \hspace{-5mm}
        % \begin{tabular}{c}
        %     \begin{tabular}{c}
        %     \includegraphics[width=\attrszgender]{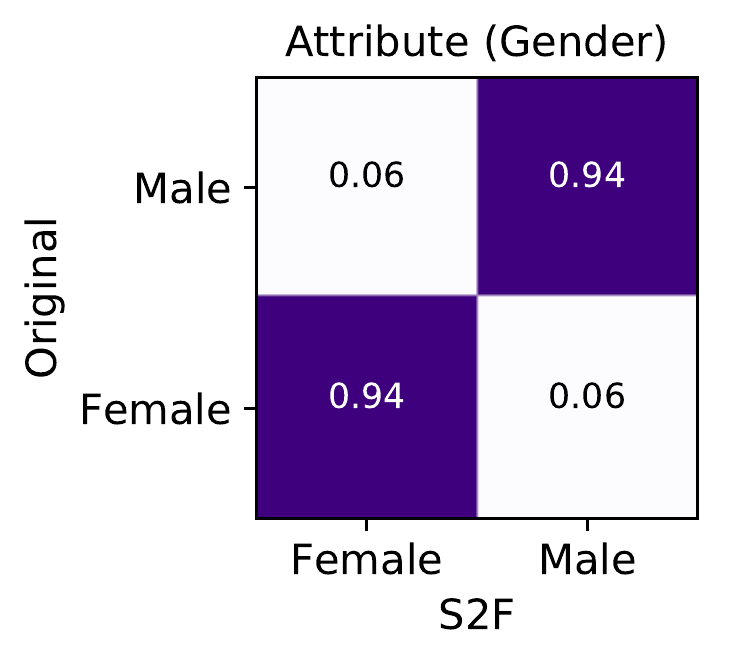}\vspace{-2mm}\\
        %     (a) \texttt{Ori-vs-S2F}\vspace{1mm} \\
        %     \includegraphics[width=\attrszgender]{figures/attr/Gender_ori_f2f.pdf}\vspace{-2mm}\\
        %     (b) \texttt{Ori-vs-F2F}
        %     \end{tabular}
        %     \begin{tabular}{c@{\hskip 0in}c}
        %     \includegraphics[width=\attrszage]{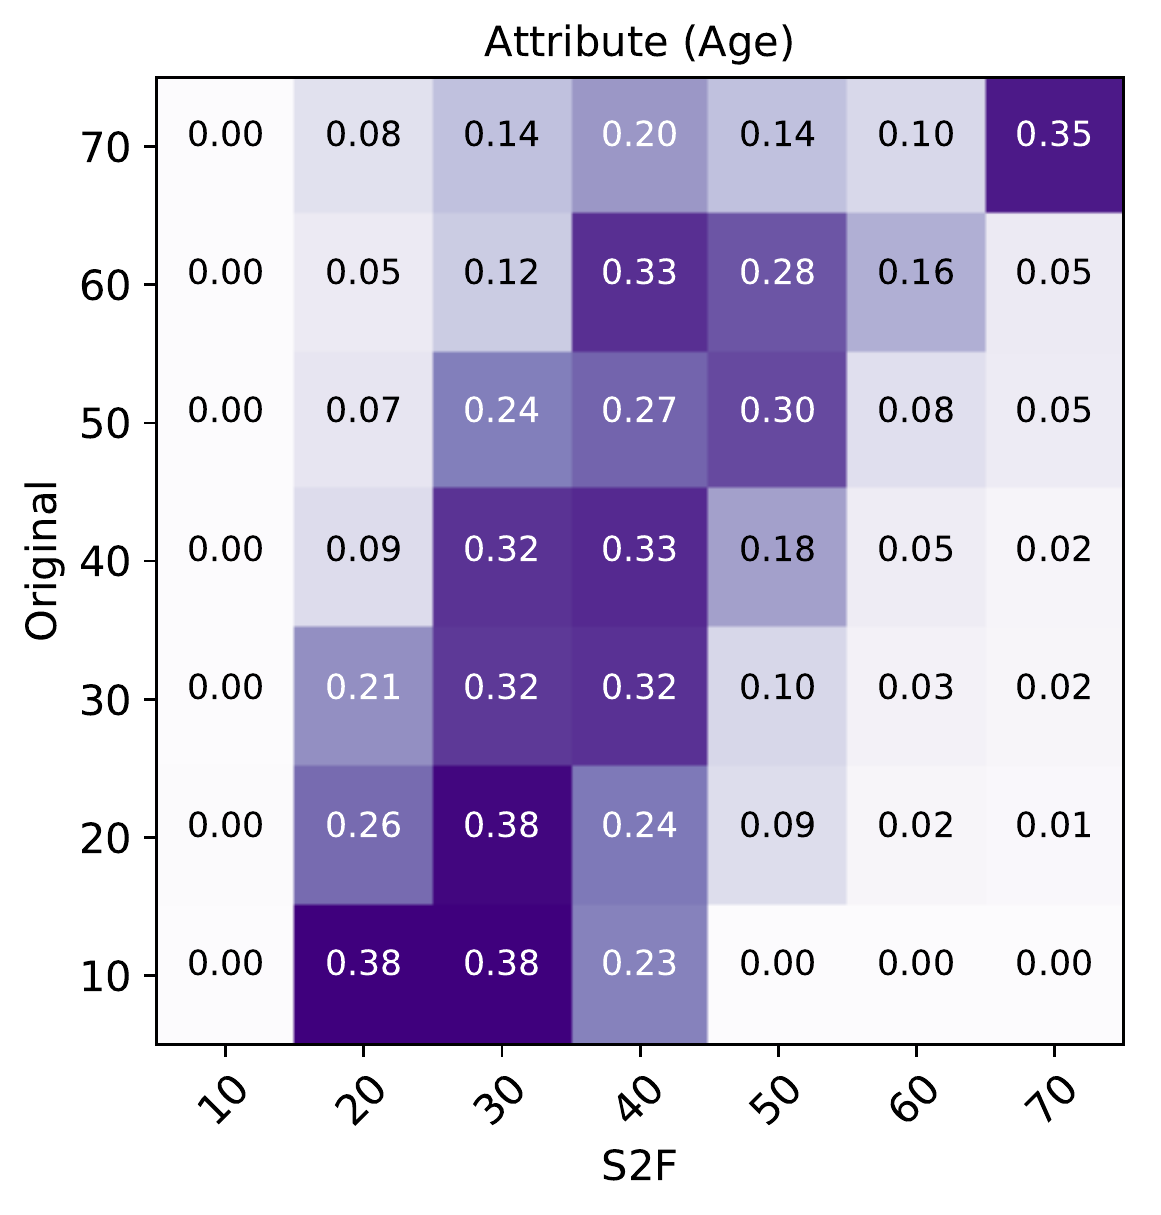}&
        %     \includegraphics[width=\attrszage]{figures/attr/Age_ori_f2f.pdf}\vspace{-2mm}\\
        %     (c) \texttt{Ori-vs-S2F} &
        %     (d) \texttt{Ori-vs-F2F}
        %     \end{tabular}\vspace{-1mm}
        % \\
        %     \begin{tabular}{c@{\hskip 0in}c}
        %     % \includegraphics[width=\attrszethnicity]{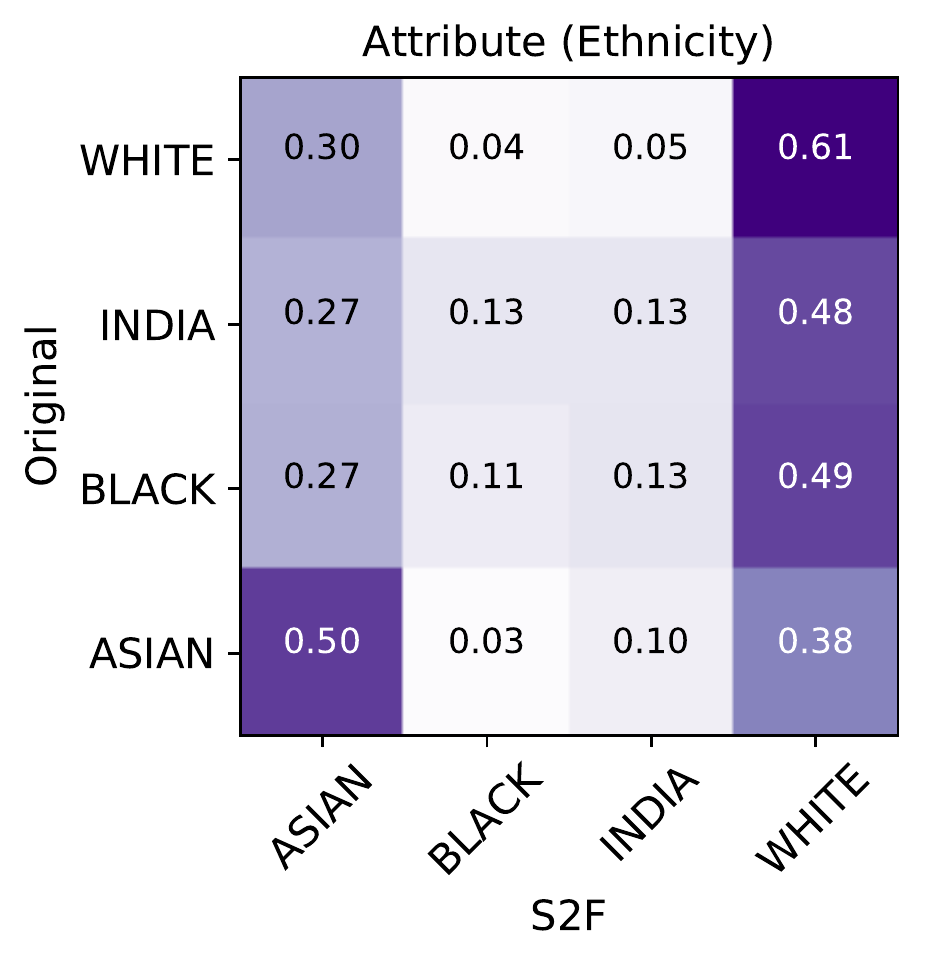}& 
        %     \includegraphics[width=\attrszethnicity]{figures/attr/Ethnicity_ori_f2f.pdf}\vspace{-2mm}\\
        %     (e) \texttt{Ori-vs-S2F}& 
        %     (f) \texttt{Ori-vs-F2F}
        %     \end{tabular}
            % \begin{tabular}{cc} %@{\hskip 0in}c
            % \multicolumn{2}{c}{
            % \includegraphics[width=0.36\linewidth]{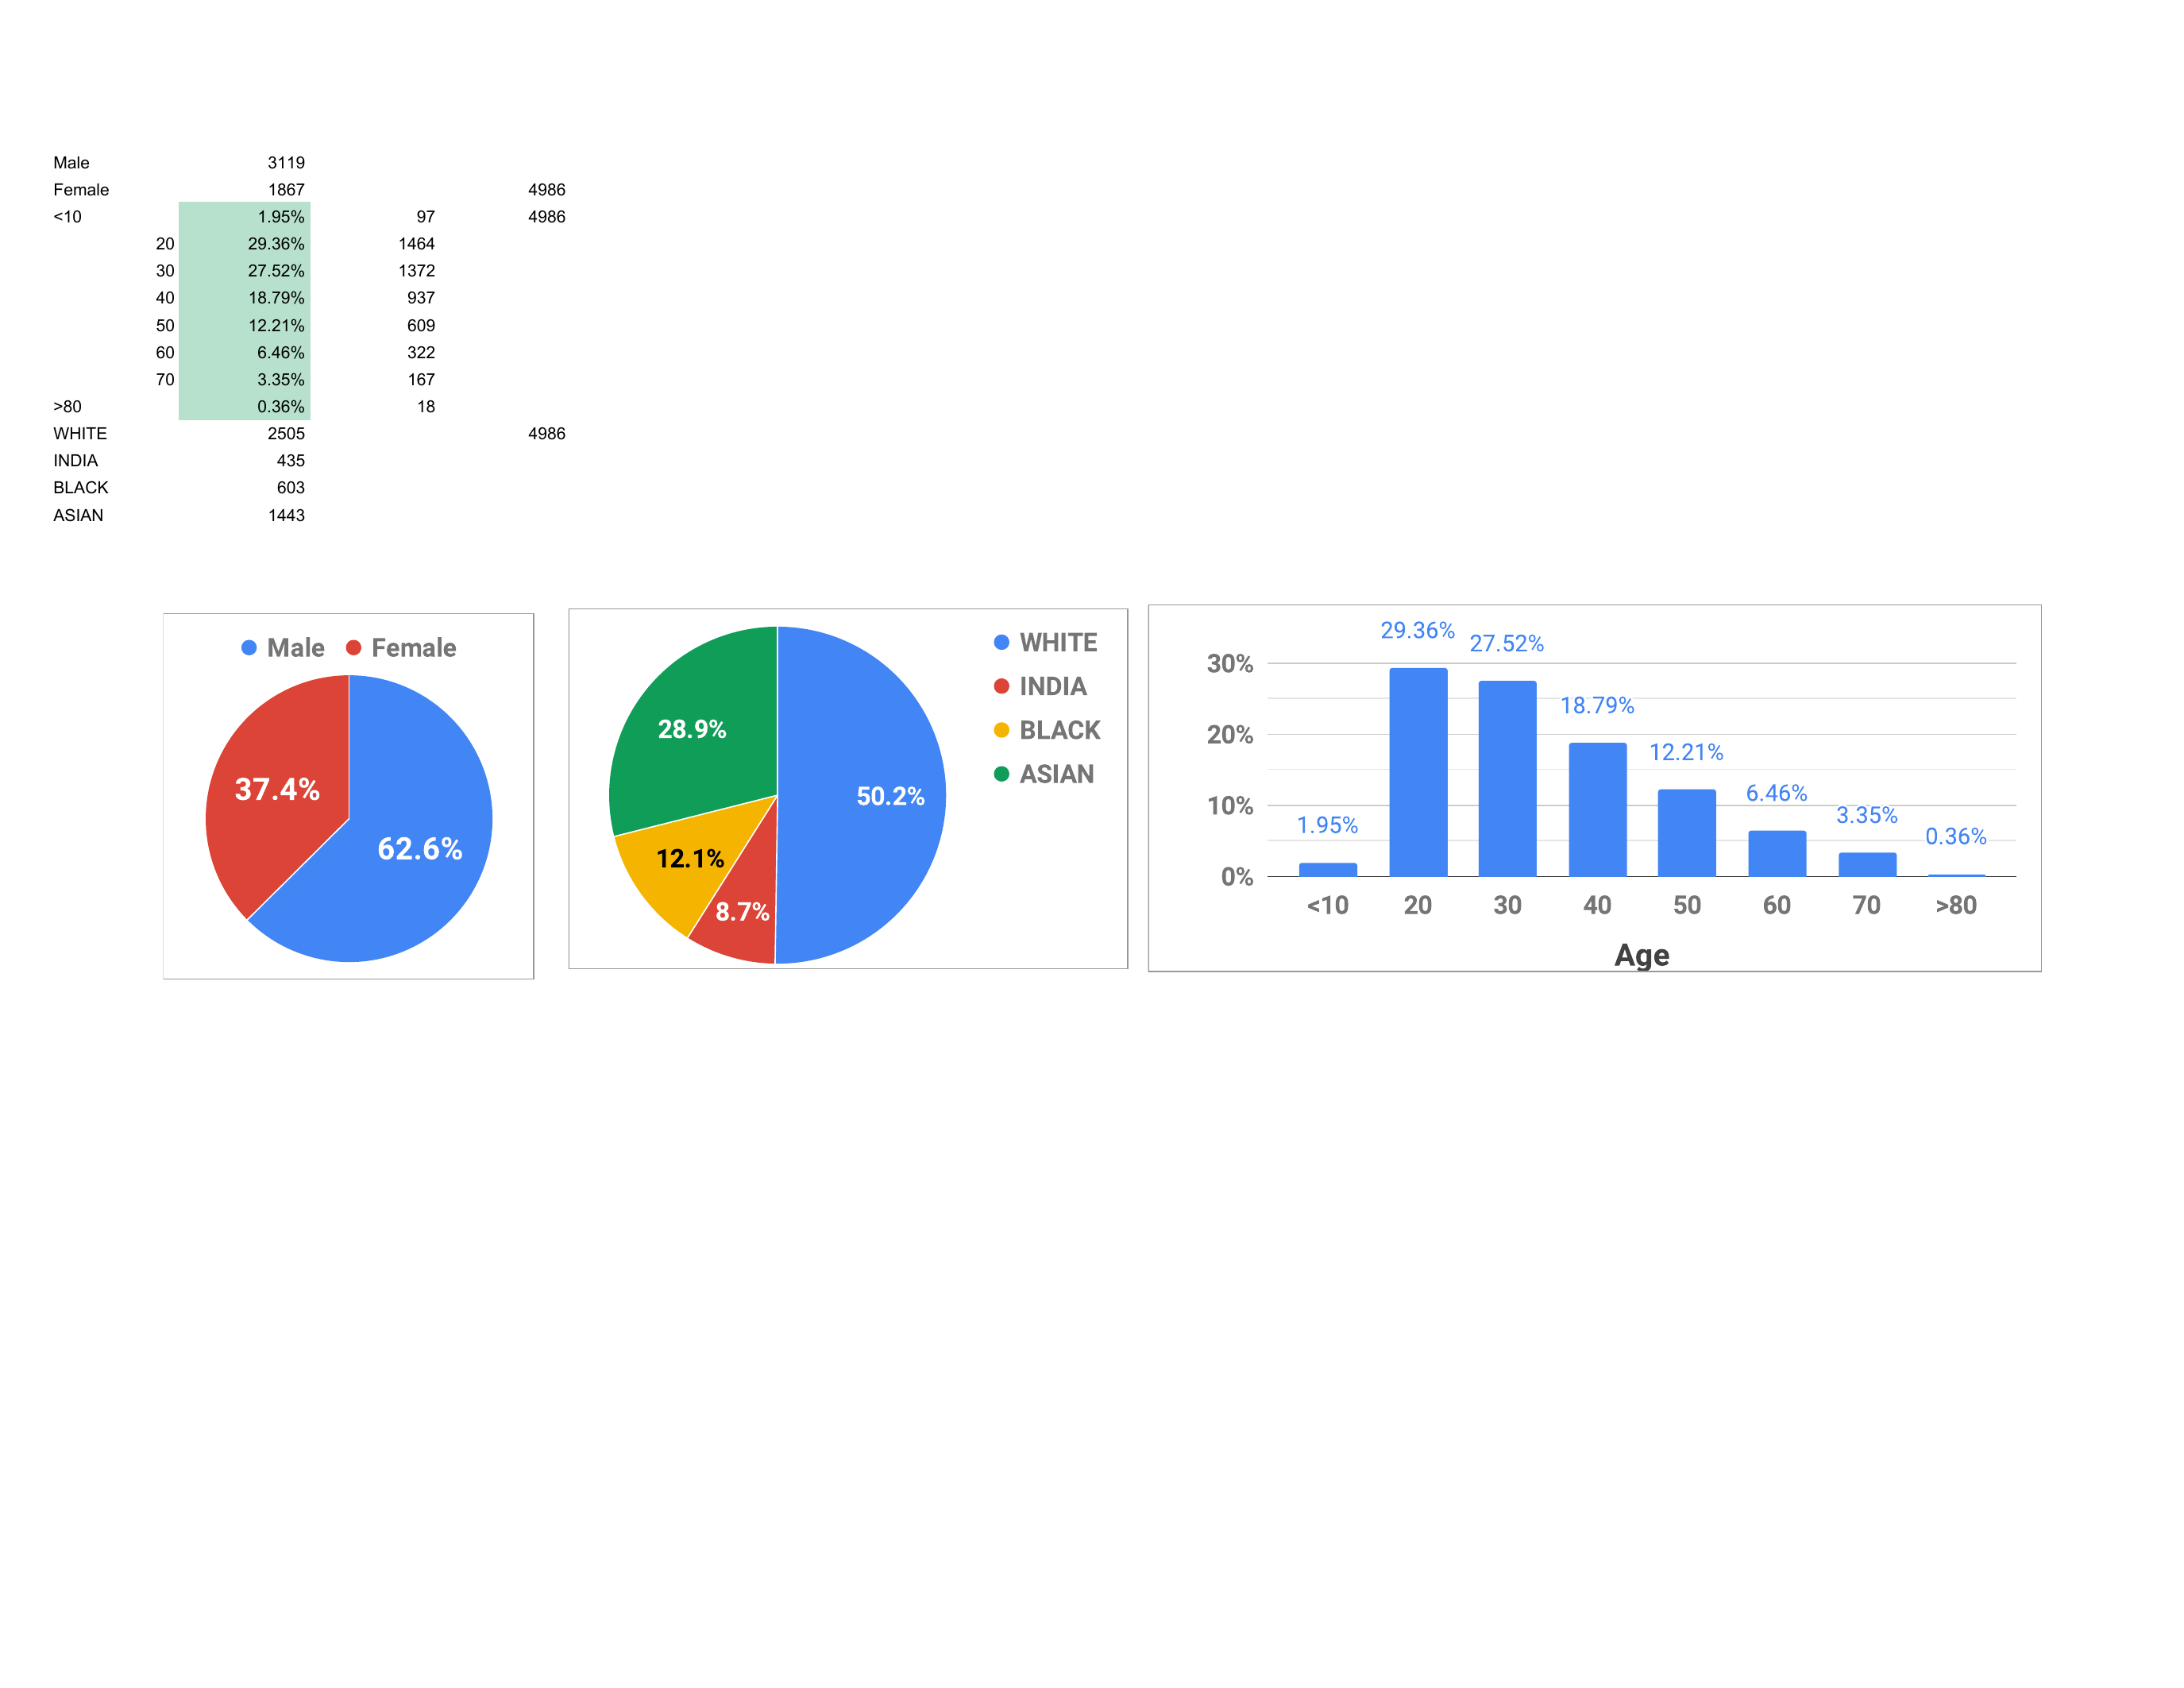}
            % }\vspace{-1mm}\\
            % \multicolumn{2}{c}{
            % \scriptsize Age
            % }\\
            % \includegraphics[height=0.12\linewidth]{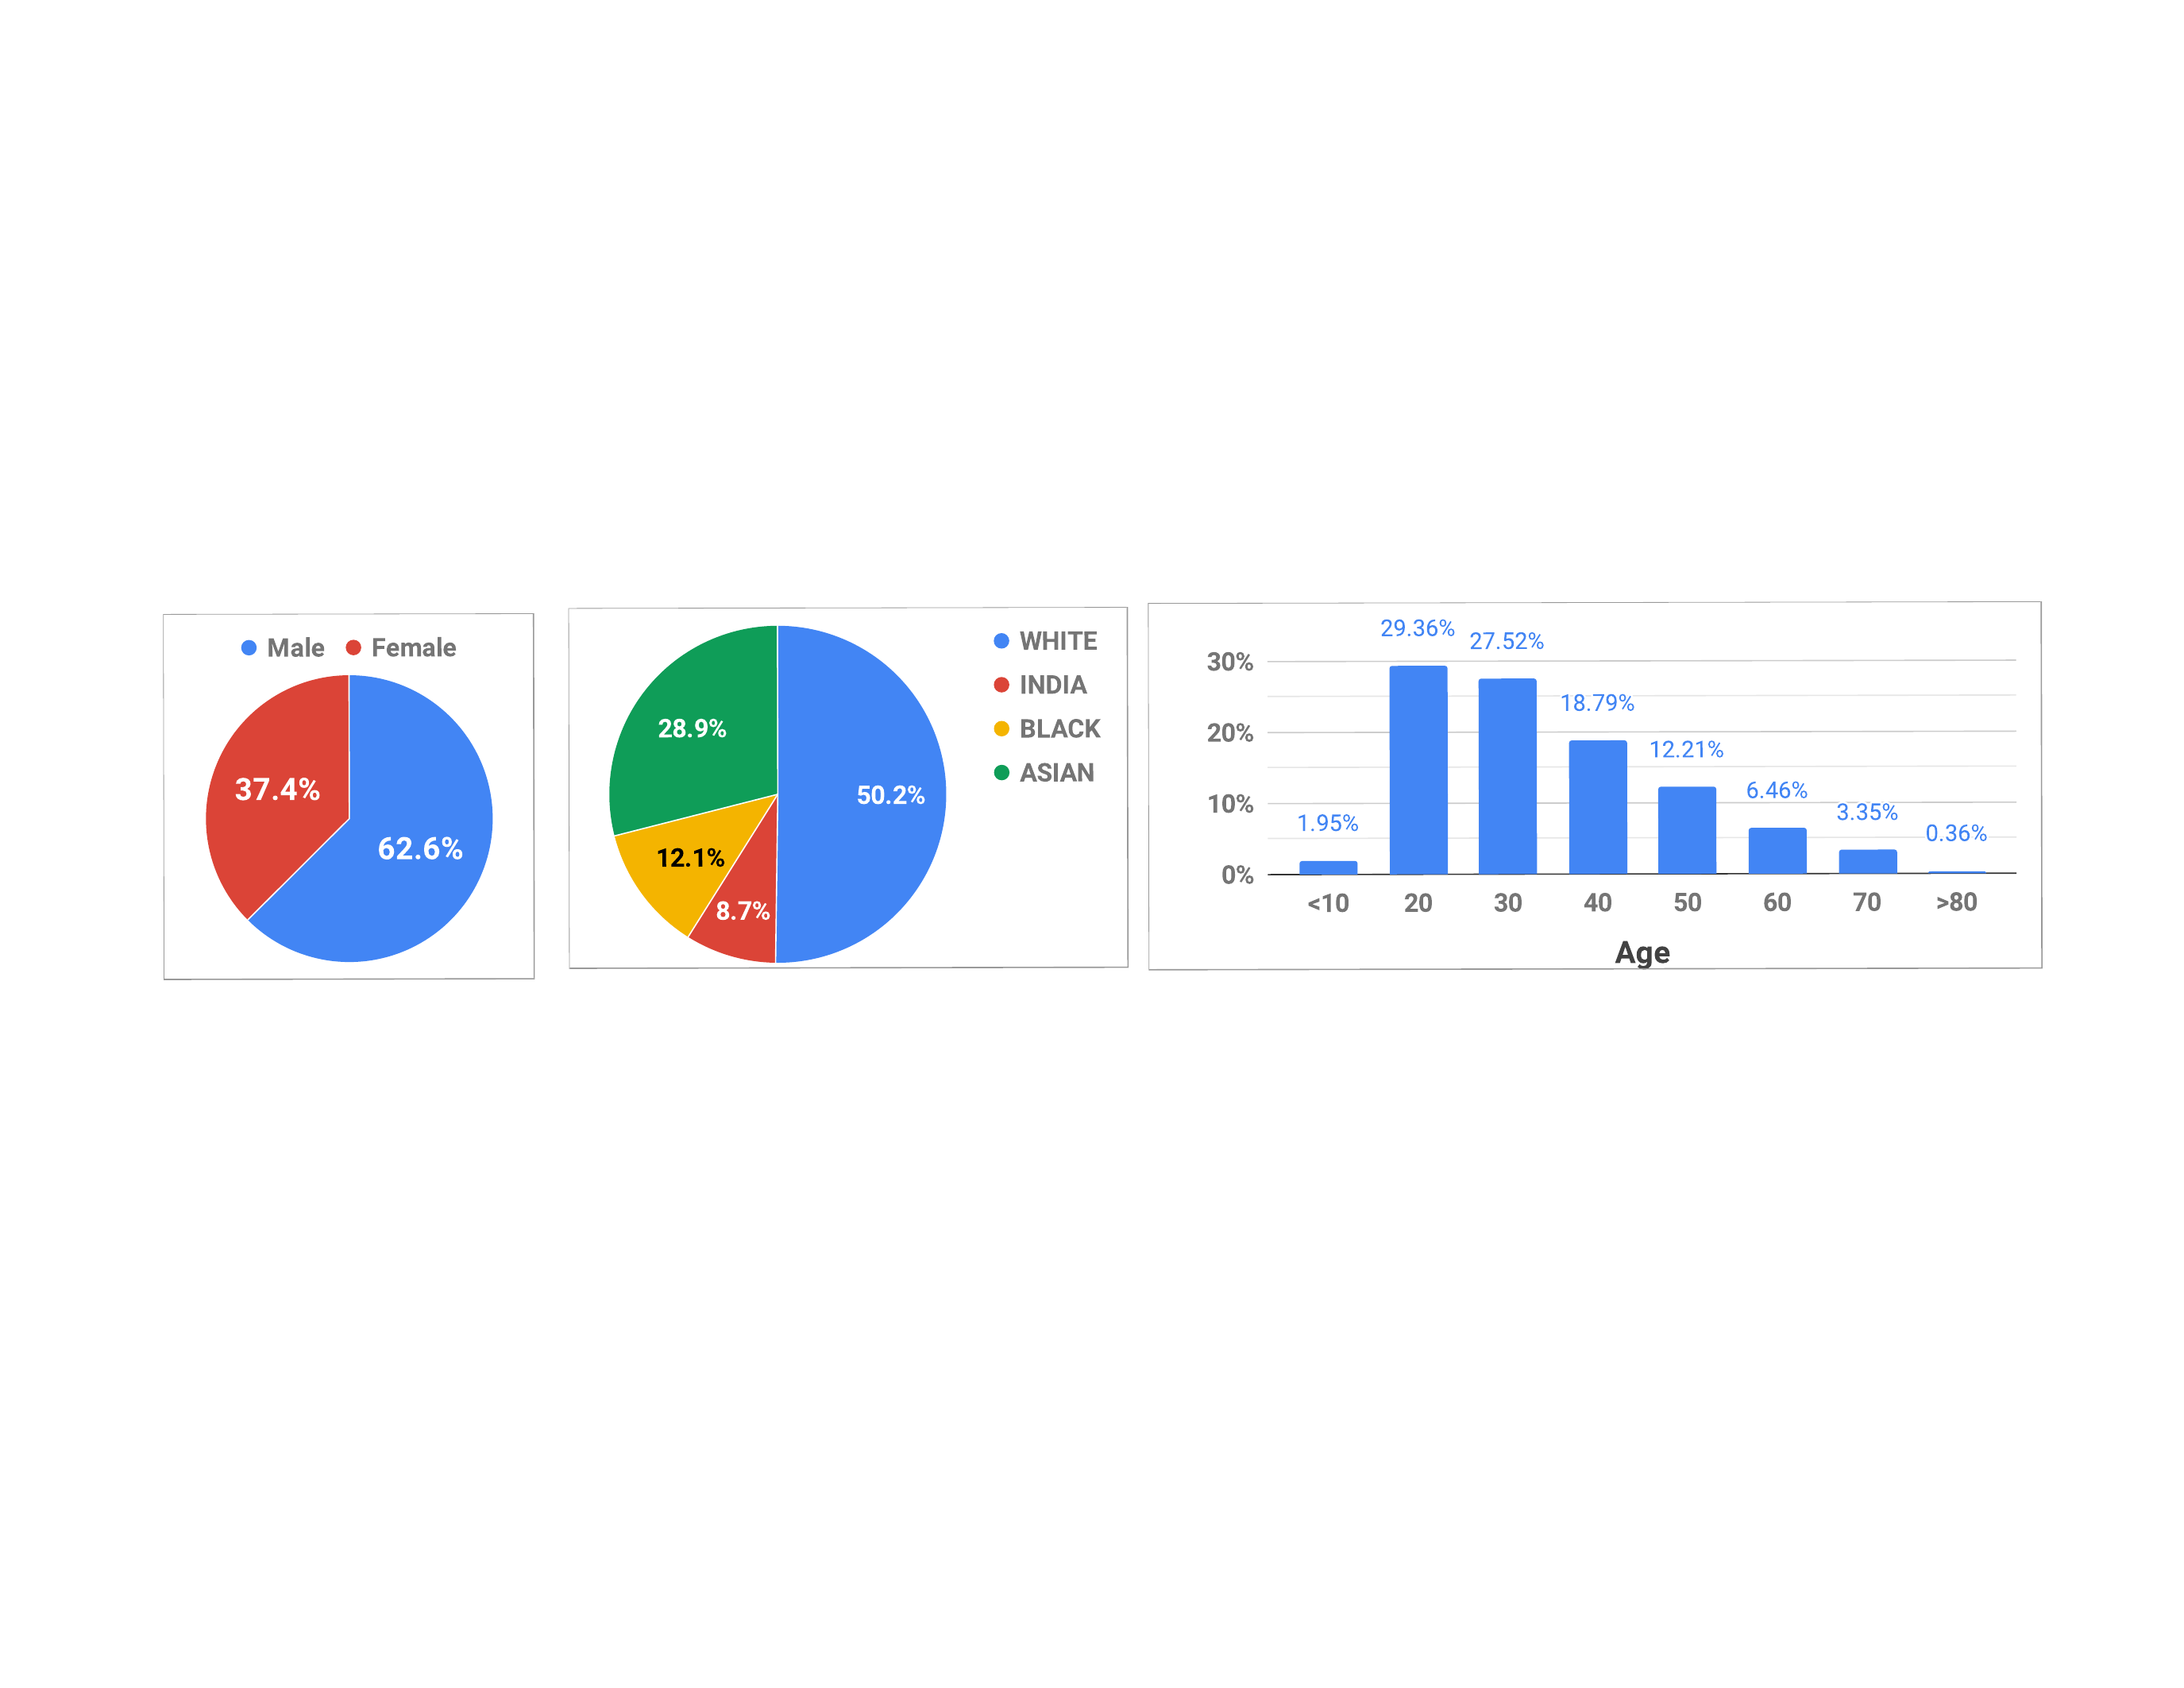}
            % % \hspace{3mm}
            % &
            % \includegraphics[height=0.12\linewidth]{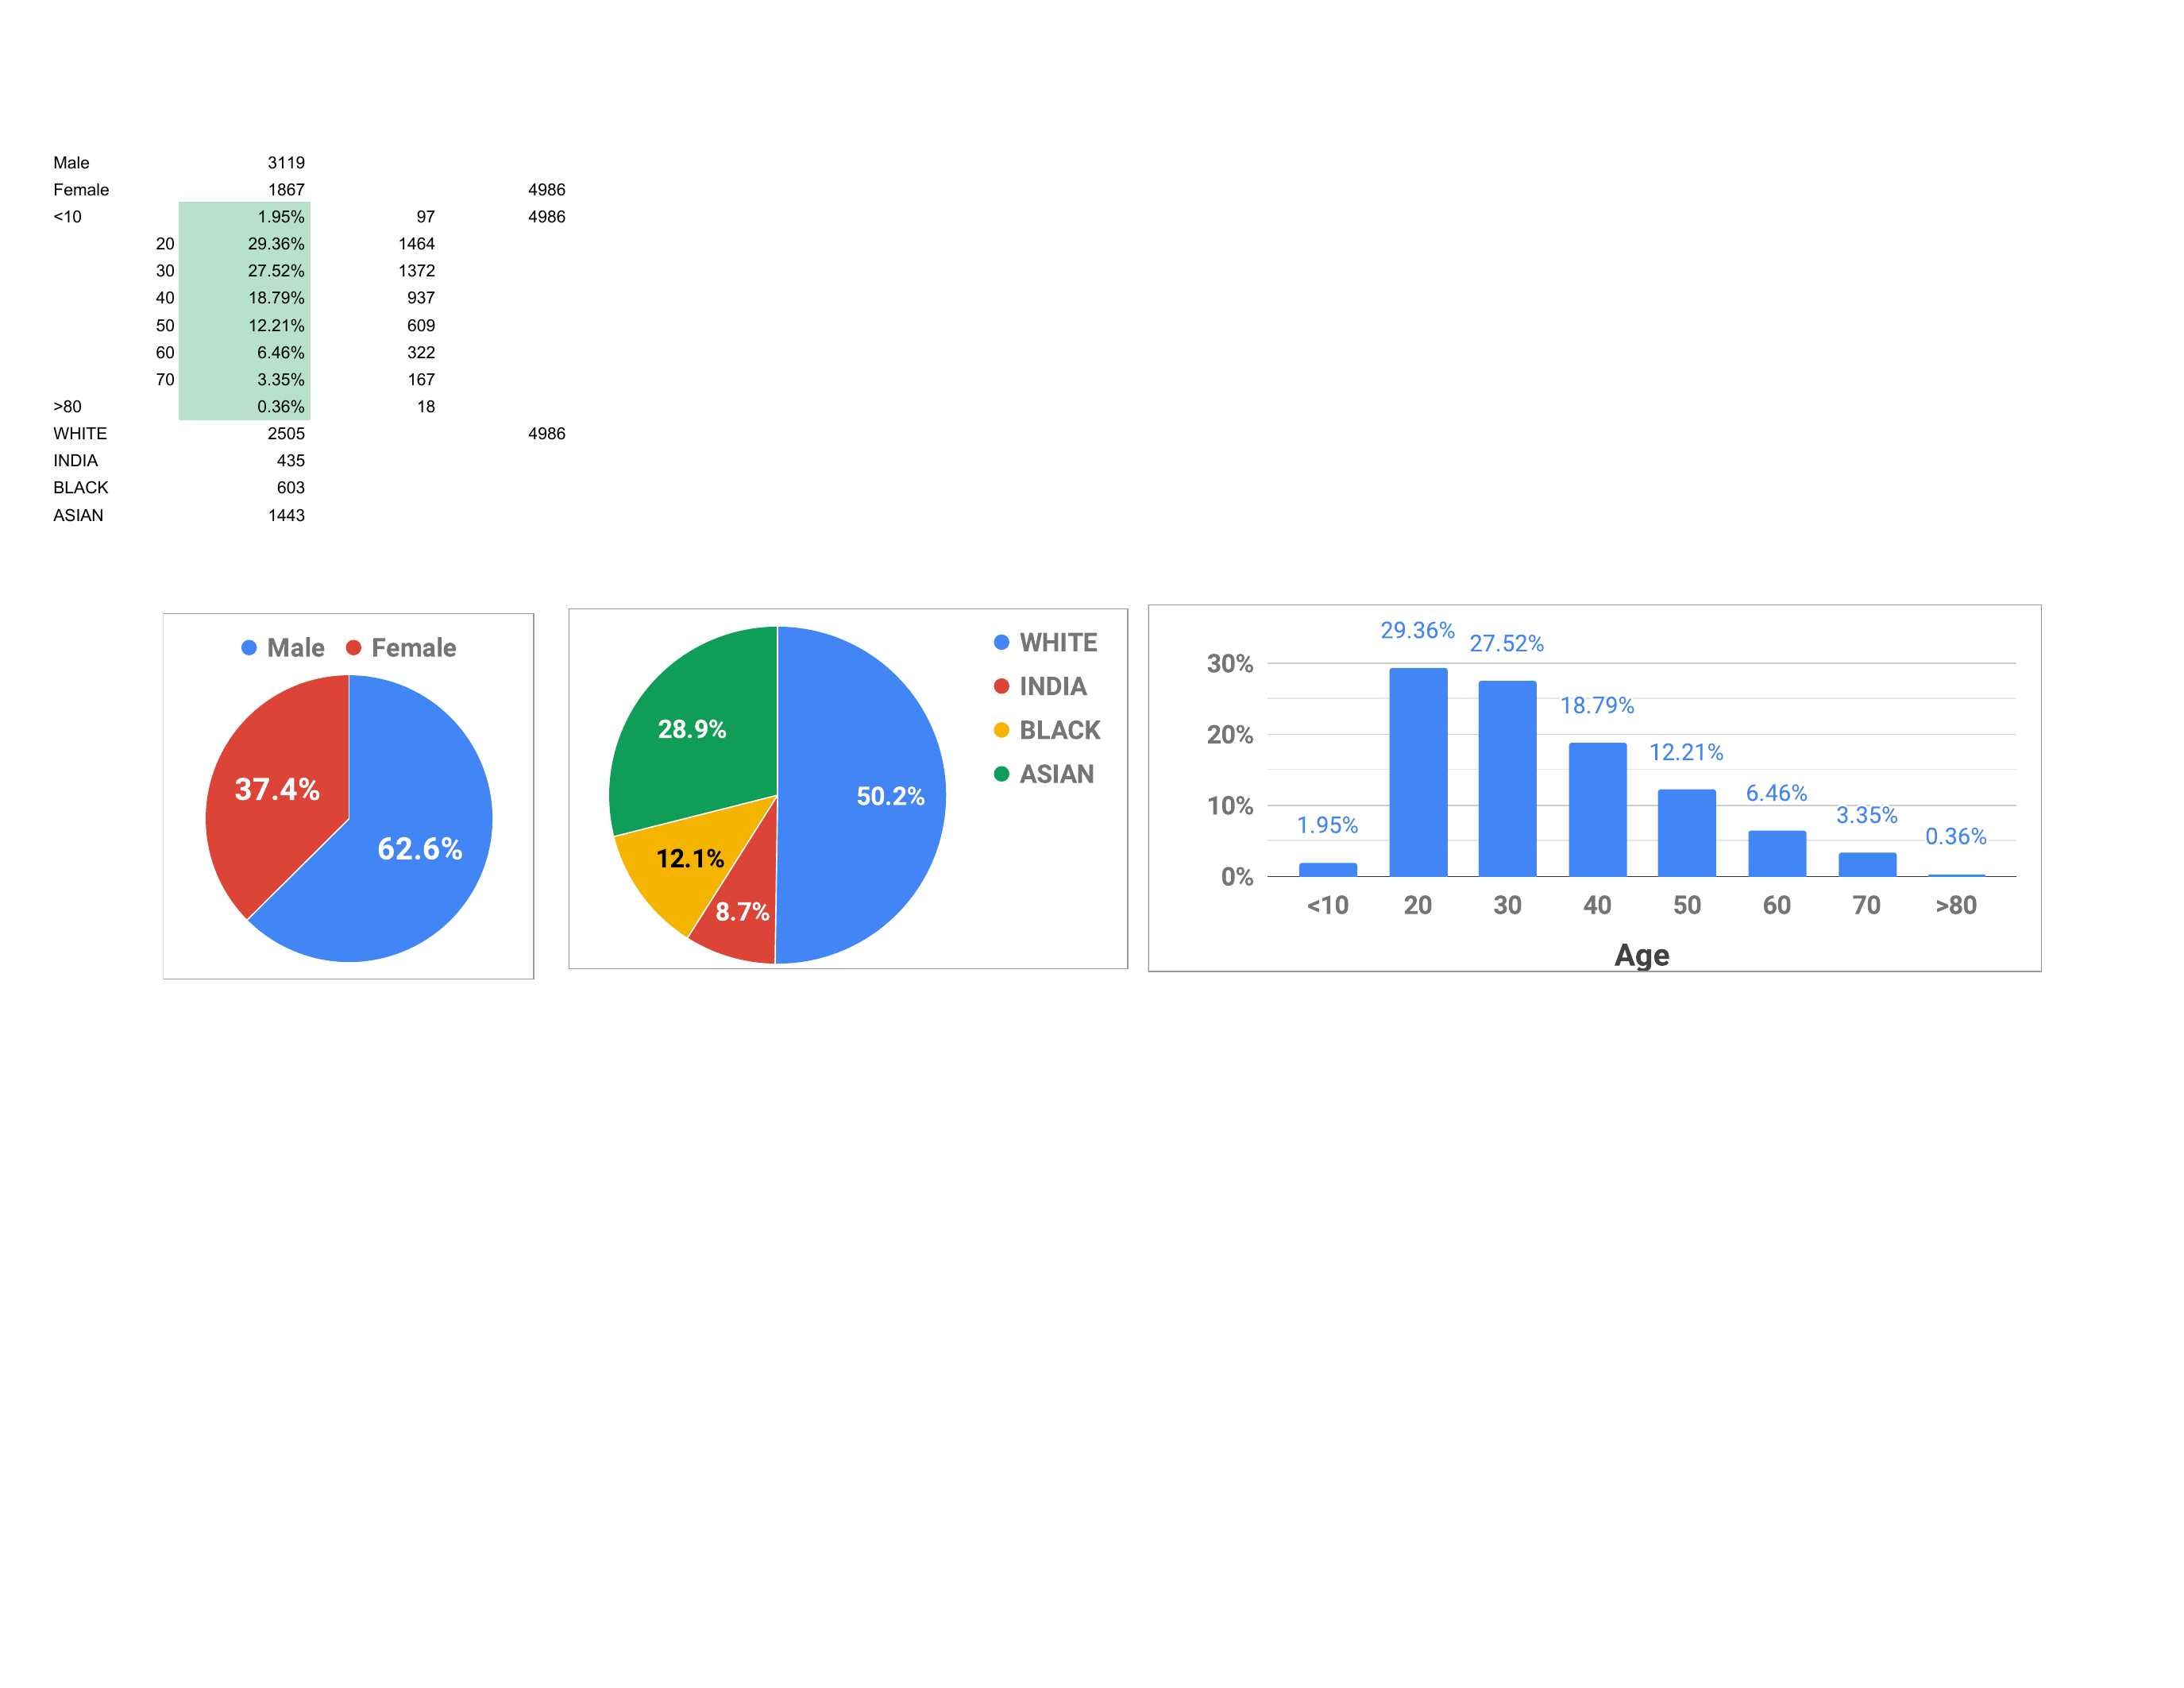}\\
            % \scriptsize Gender & \scriptsize Ethnicity\vspace{1mm}\\
            % \multicolumn{2}{c}{(g) AVSpeech training set statistics}
            % \end{tabular}
            % \hspace{-2mm}
        % \end{tabular}
}
\vspace{1mm}
    \caption{Attribute confusion matrix between original face image and face reconstruction from face feature (F2F). 
    This is presented for reference to see the performance deviation sourced by the face decoder module.
    We compute the confusion matrix with row-wise normalization, where strong diagonal tendency indicates a better performance. 
    }
    \label{fig:attr_eval_f2f}
    \afterfig
\end{figure*}

\subsection*{t-SNE visualization on AVSpeech}

% \subsection{Visualizing the Learned Face Features}
% \noindent
To gain more insights on our predicted features, we visualize 2-D t-SNE plot~\cite{maaten2008visualizing} of the features
% to reduce their dimensionality and visualize them 
in Fig.~\ref{fig:tsne}, whereby we compare our features with 
% this with the same visualization produced using 
the VGG-Face features computed directly from the original images.
We use the VoxCeleb audiovisual dataset~\cite{Nagrani2017}, which consists of short video clips of celebrities speaking. 
In addition to the gender annotations accompanying the dataset, we used the age and ethnicity annotations from Kim et al.~\cite{kim2018on} that are given on the same dataset.

% In Fig.~\ref{fig:tsne}, we show the resulting 2-D maps for the original face features (red boxes) and our predicted face features from voice (green boxes). 
% In each plot, we consider a different set of attributes (age, gender, ethnicity) and color-code each sample with its associated attribute. 
Note that the projected features from image (red boxes) form small clusters, each corresponding to a different identity (since VGG-Face is trained for face identification).
%Note that when features are projected by t-SNE, no attribute information is used.  
% We projected those features onto 2-D spaces computed for each type of feature using t-SNE~\cite{maaten2008visualizing}. The resulting visulizations are shown in \figref{tsne}. Note that the projected face features form small clusters because the VGG-Face model is trained for face identification, and so each of those small clusters likely corresponds to a different identity. 
%However, the face features visualization lacks global structures compared to the t-SNE of our voice features. For example, 
As can be seen, gender is the major distinctive feature captured by our learned feature from voice, dividing the space into two separated clusters. In addition, we can observe a smooth transition between age groups in our face features from voice. However, there is no clear structure in our features 
% when it comes to determining 
regarding ethnicity.
% , as well as native vs. non-native English speakers. 
These properties are better captured by the face features computed from images. Note that the VoxCeleb dataset includes celebrities and public figures, which may not be a good representation of the general population in terms of ethnicity, language, and accents. Overall, these visualizations agree with our numerical analysis.

% \begin{strip}
\begin{figure*}[t]
% \InsertBoxC{
    \centering
    % \vspace{-.2in}
    \addtocounter{figure}{1}% Re-establish correct figure number
    \includegraphics[width=\textwidth]{figures/tsne/tsne_voxceleb_tali.pdf}
    % }
    \caption{\textbf{Visualizing the feature space.}  t-SNE visualizations % (features projected onto a 2-D space)
    for the face features obtained from the original images by feeding them into VGG-Face (red boxes), and for the features predicted by our voice encoder (green boxes). We use the same computed projections for each feature type, but in each plot color-code the data points using a different attribute (from left to right: gender, age, and ethnicity).
   We use the VoxCeleb dataset and the human-labeled attribute annotations from Kim et al.~\cite{kim2018on} (not used for training). Notice for example how gender is the major distinctive feature in our learned feature space, dividing the space into two separated clusters. See more discussion in the text.}
    \label{fig:tsne}\afterfig
\end{figure*}
% \end{strip}

\oh{I will work on the supplementary}
\figref{tsne_supple}

\ifdefined\arxivversion
\vspace{1mm}
\else
   \input{sec4add2_results.tex}
\fi

\begin{figure*}[t]
  % macros for the t-sne plots
  \newcommand{\addtext}[2]{\parbox{#1}{\centering\small{}#2}}
  \newcommand{\addvtext}[3]{\begin{sideways}\parbox[c][#1][c]{#2}{\centering\small{}#3}\end{sideways}}
  \newcommand{\capcolwidth}{.02\linewidth}
  \newcommand{\capcolheight}{.16\linewidth}
  \newcommand{\colwidth}{.15\linewidth}
  \newcommand{\colgap}{}
  % figure starts
  \centering
  \addvtext{\capcolwidth}{\capcolheight}{Face features}\colgap%
  \includegraphics[width=\colwidth]{figures/tsne/tsne_feat_f_4k_50_age}\colgap%
  \includegraphics[width=\colwidth]{figures/tsne/tsne_feat_f_4k_50_gender}\colgap%
  \includegraphics[width=\colwidth]{figures/tsne/tsne_feat_f_4k_50_ethnicity}\qquad%
  \includegraphics[width=\colwidth]{figures/tsne/avspeech/tsne_feat_f_4k_50_age}\colgap%
  \includegraphics[width=\colwidth]{figures/tsne/avspeech/tsne_feat_f_4k_50_gender}\colgap%
  \includegraphics[width=\colwidth]{figures/tsne/avspeech/tsne_feat_f_4k_50_ethnicity}\\%
  \addvtext{\capcolwidth}{\capcolheight}{Voice features}\colgap%
  \includegraphics[width=\colwidth]{figures/tsne/tsne_feat_v_4k_50_age}\colgap%
  \includegraphics[width=\colwidth]{figures/tsne/tsne_feat_v_4k_50_gender}\colgap%
  \includegraphics[width=\colwidth]{figures/tsne/tsne_feat_v_4k_50_ethnicity}\qquad%
  \includegraphics[width=\colwidth]{figures/tsne/avspeech/tsne_feat_v_4k_50_age}\colgap%
  \includegraphics[width=\colwidth]{figures/tsne/avspeech/tsne_feat_v_4k_50_gender}\colgap%
  \includegraphics[width=\colwidth]{figures/tsne/avspeech/tsne_feat_v_4k_50_ethnicity}\\[-2mm]%
  \addvtext{\capcolwidth}{.01\linewidth}{}\colgap%
  \addtext{\colwidth}{Age}\colgap%
  \addtext{\colwidth}{Gender}\colgap%
  \addtext{\colwidth}{Ethnicity}\qquad%
  \addtext{\colwidth}{Age}\colgap%
  \addtext{\colwidth}{Gender}\colgap%
  \addtext{\colwidth}{Ethnicity}\\[2mm]%
  \addtext{.45\linewidth}{VoxCeleb dataset}\qquad
  \addtext{.45\linewidth}{AVSpeech dataset}\\[2mm]
  \caption{\textbf{t-SNE visualization of the learned feature space.} 
   Face features obtained from the original images by feeding them into VGG-Face (top row) and the learned \emph{voice features} predicted by our voice encoder (bottom row) are visualized.
   For each type of feature (row), all plots use the same computed t-SNE embedding, where in each plot (column) the data points are color-coded using a different attribute (from left to right: age, gender, and ethnicity).
   For the samples, we use the VoxCeleb dataset and take its attribute annotations from Kim et al.~\cite{kim2018on}.
   Note that these attributes were not used for training.
%   t-SNE visualizations~\cite{maaten2008visualizing} of face features obtained from the original images by feeding them into the VGG-Face model (top row) and the learned \emph{voice features} predicted by our voice encoder (bottom row), of 656 random samples from the VoxCeleb dataset (left half) and random samples from the AVSpeech dataset (right half). For each type of feature (row), all plots use the same computed t-SNE embedding, where in each plot (column) the data points are color-coded using a different attribute (from left to right: age, gender, and ethnicity). The attribute annotations are taken from Kim et al.~\cite{kim2018on} and generated by Face++~\cite{face++} for VoxCeleb and AVSpeech, respectively. Note that these attributes were not used for training.
  % \oh{Changil, do the age tsnes have continous values? It looks discrete. Could you check whether it is up-to-date one?    Also, I think we can just take 4k feature with age and gender for the main paper, and put the others in the supplementary material.    And the ethnicity tsne of voice feature seems not good to report. Reviewers may mislead that our method cannot parse ethnicity, but in the other results, it is not true. How do you think?}
  % \changil{What to show? Only gender and age? I'd remove the language column that's the least informative, but leave the ethnicity. Indeed the voice features do not seem very distinctive about the ethnicity, do they?}
  }
  \label{fig:tsne_supple}
\end{figure*}
